# Supplementary material for: VLMAE: Vision-Language Masked Autoencoder
Source: arXiv:2208.09374 source file (2022-08-19)
Supplement: Supplementary file 1 [file supp_vg.pdf]

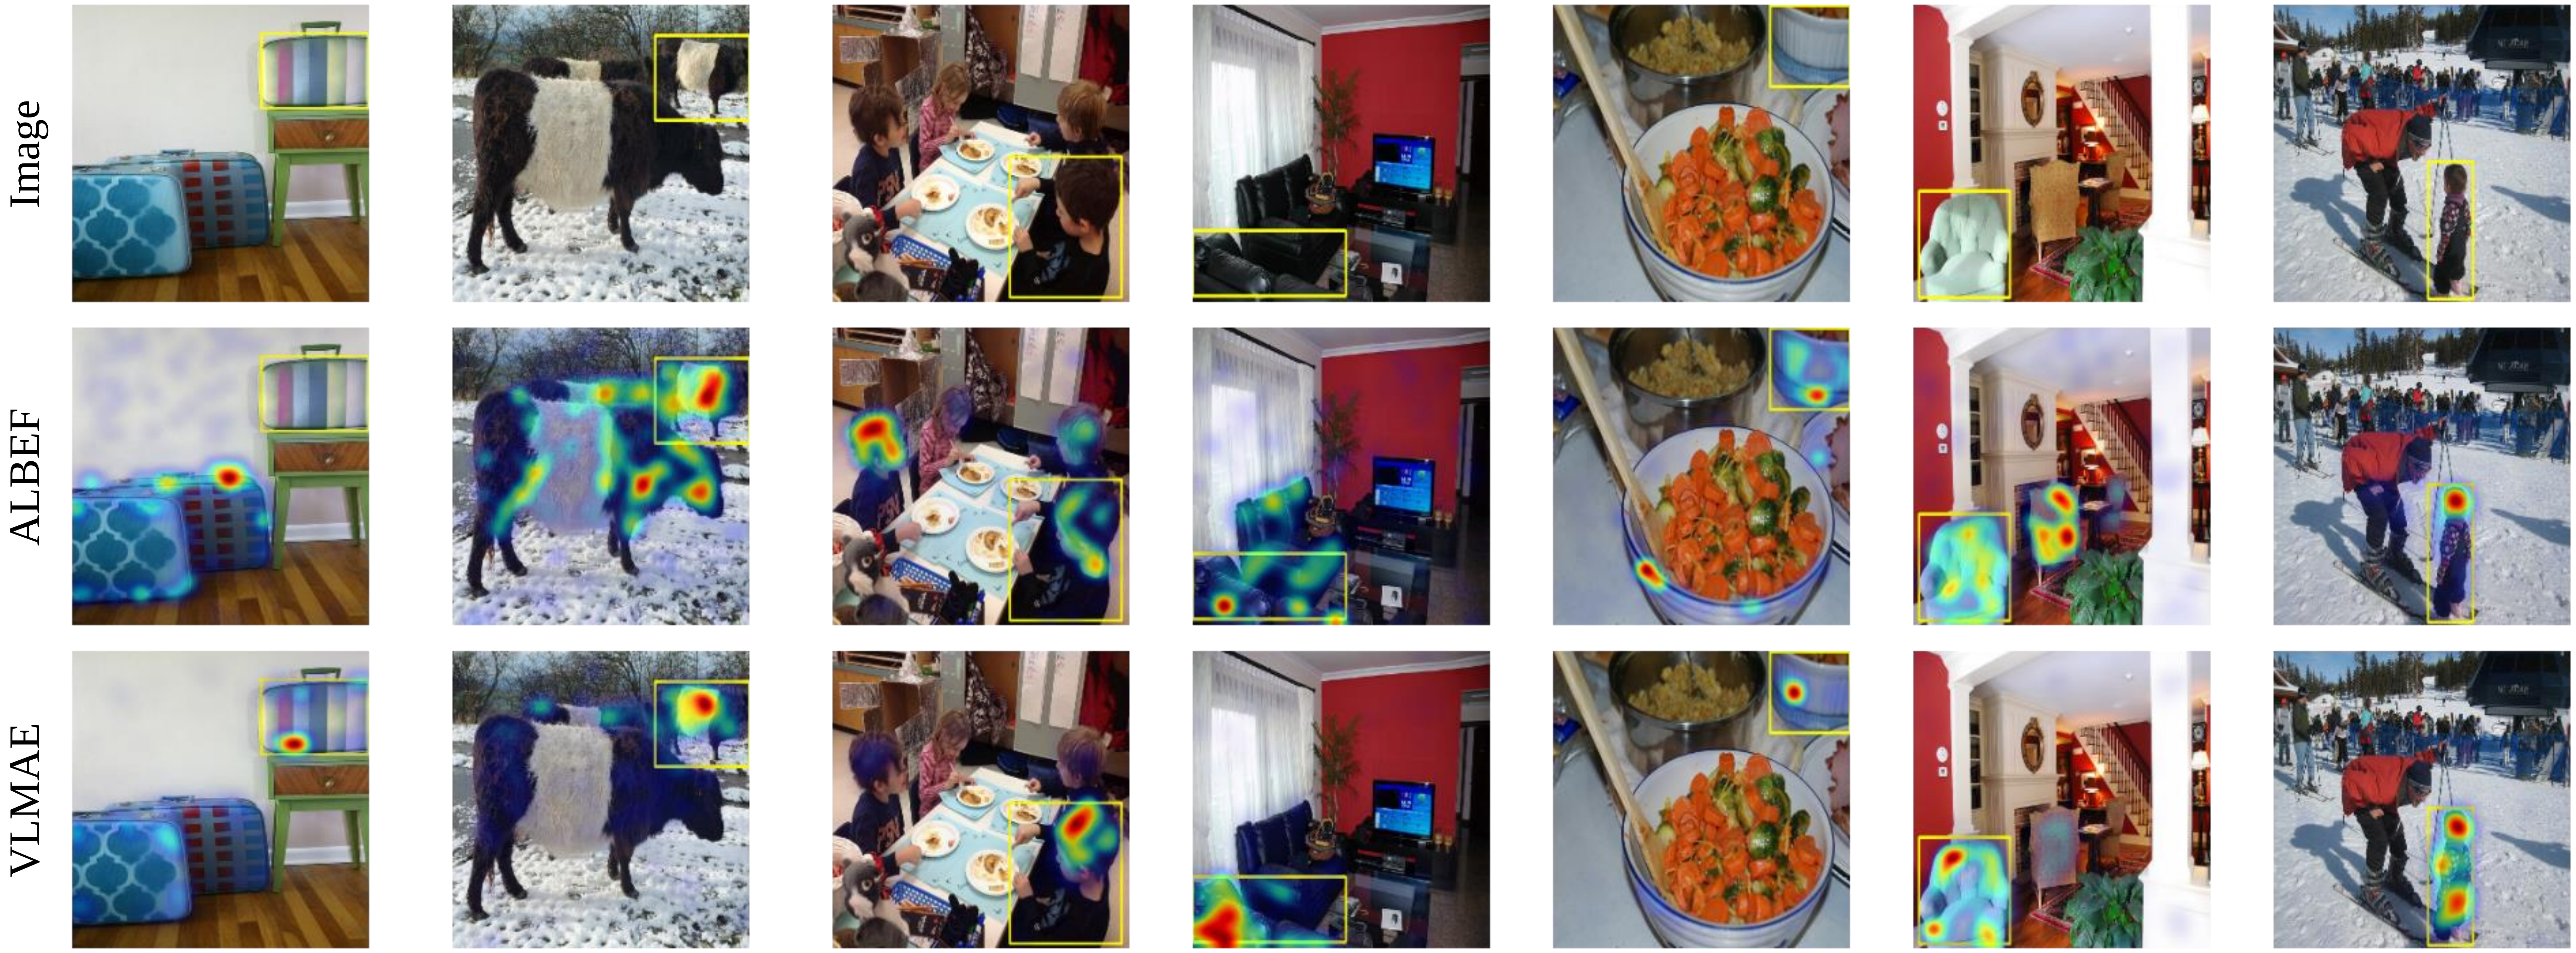


(a) Bag highest. (b) Upper corner animal. (c) Dark haired boy rightest us. (d) Black couch partial in corner. (e) White bowl with vertical stripes. (f) Green chair. (g) The kid.

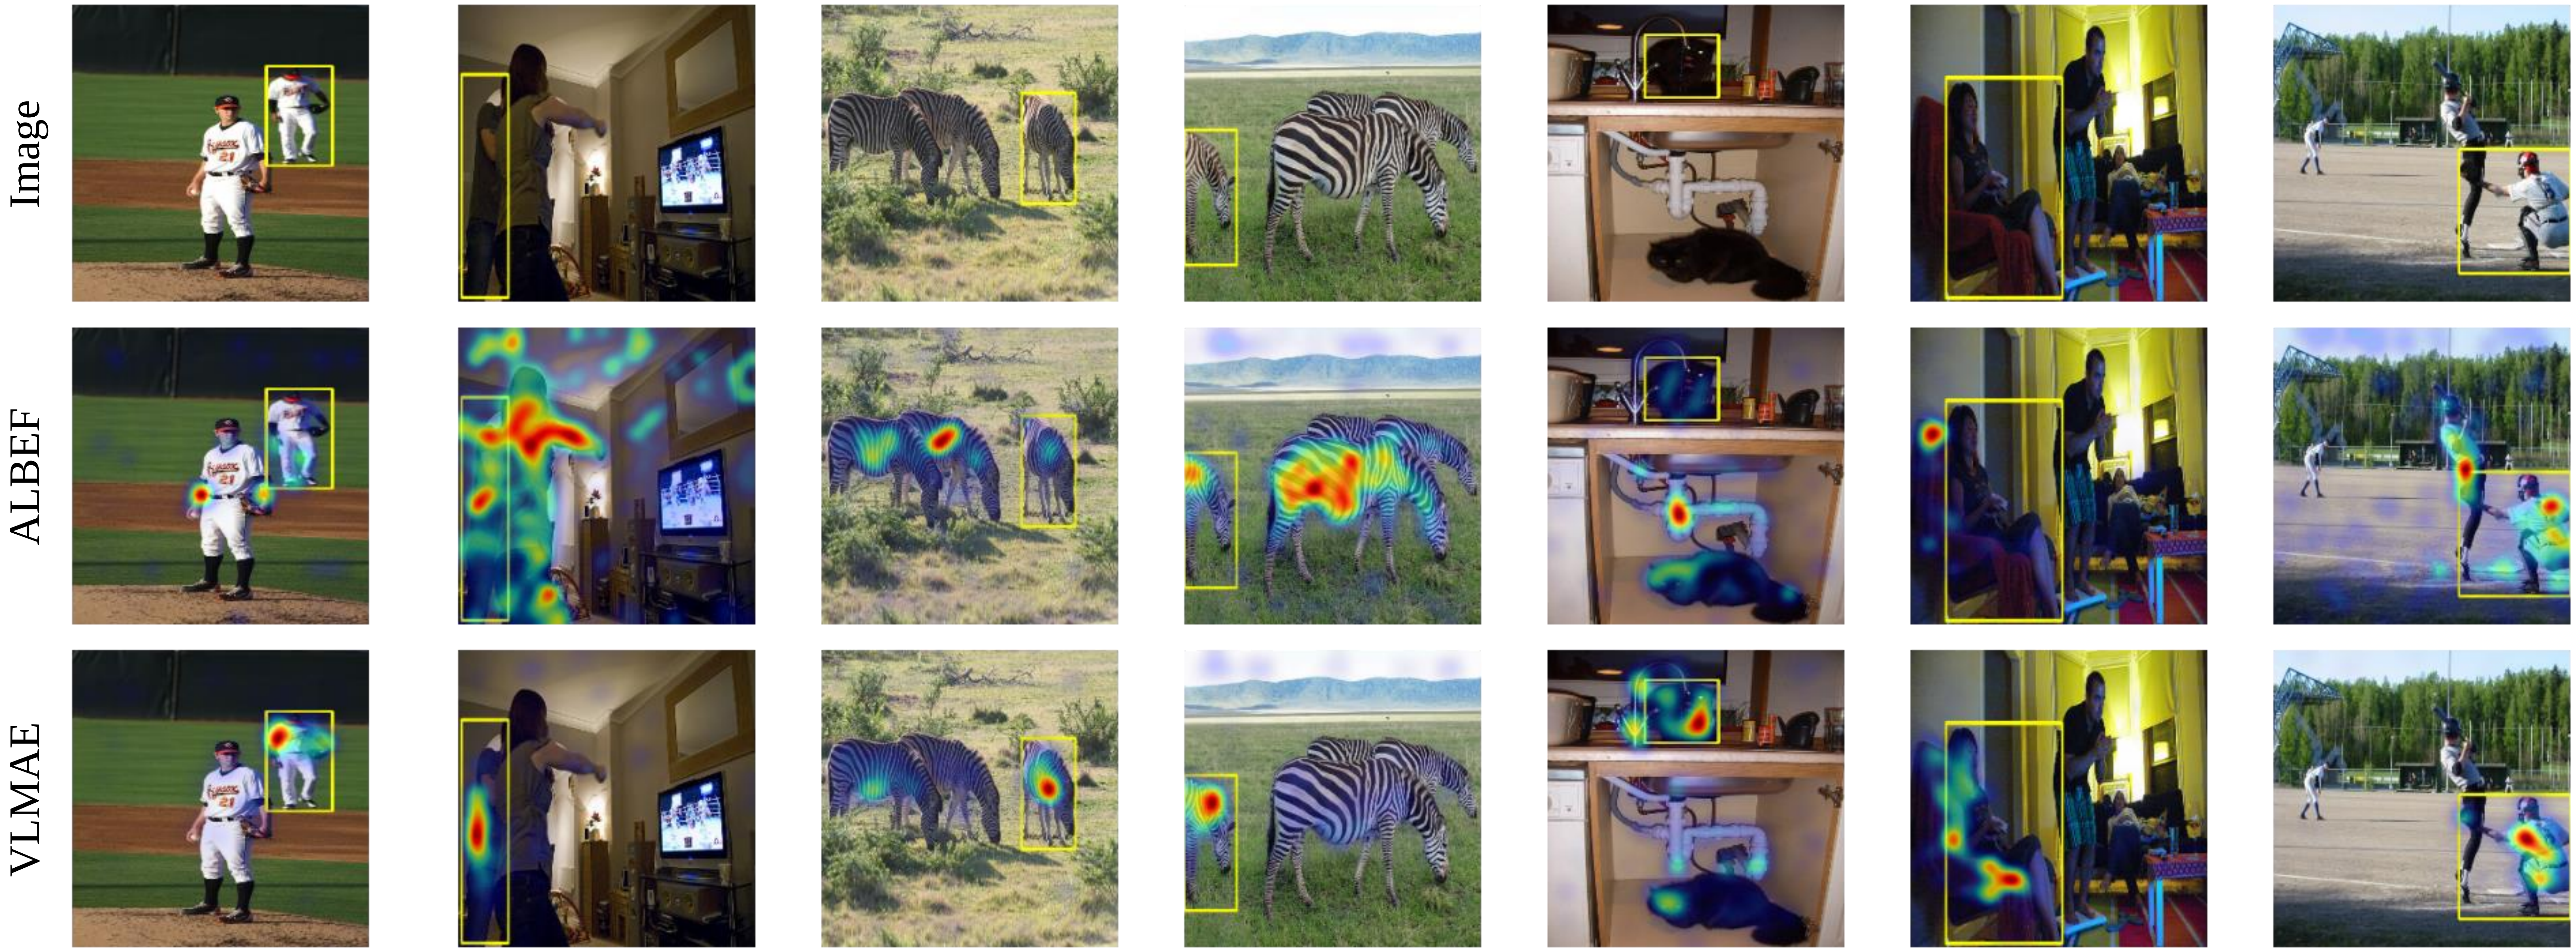


(h) Man with head down. (i) Person you cant see much. (j) Zebra by himself. (k) Half a zebra. (l) Cat by faucet. (m) Woman sitting on the red sofa. (n) Catcher.

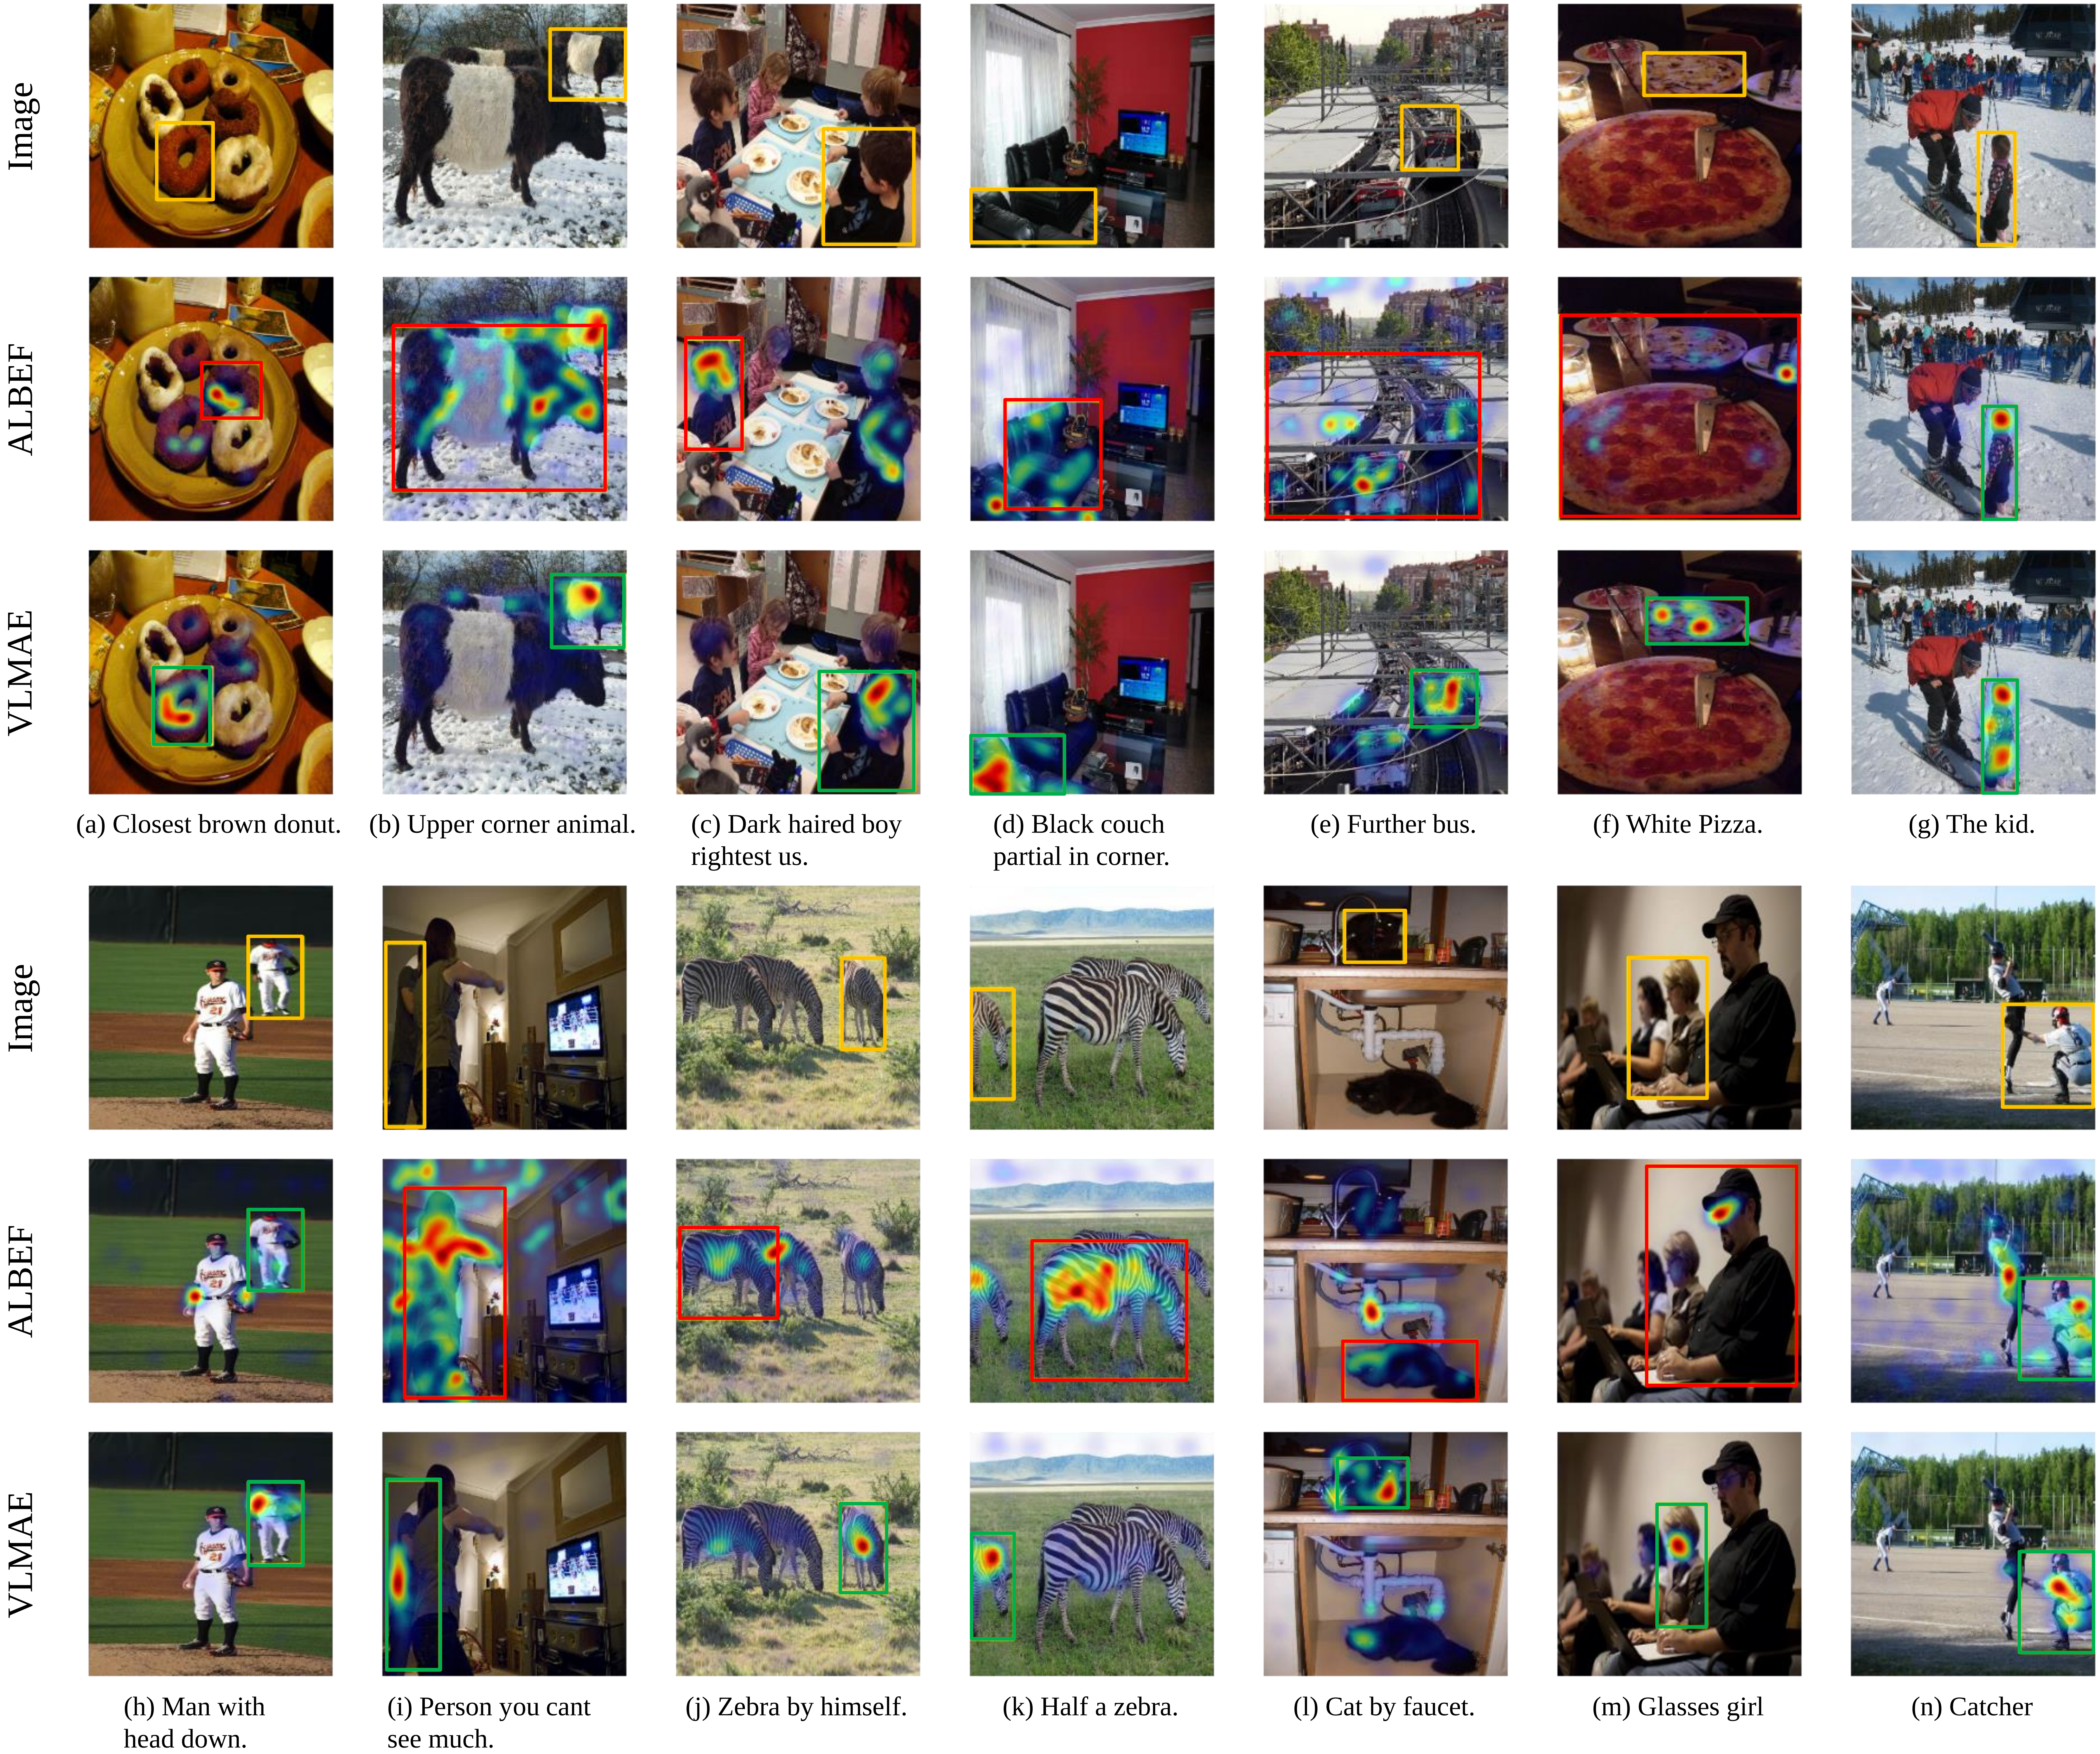
Image
ALBEF
VLMAE
(a) Closest brown donut.
(b) Upper corner animal.
(c) Dark haired boy rightest us.
(d) Black couch partial in corner.
(e) Further bus.
(f) White Pizza.
(g) The kid.
Image
ALBEF
VLMAE
(h) Man with head down.
(i) Person you cant see much.
(j) Zebra by himself.
(k) Half a zebra.
(l) Cat by faucet.
(m) Glasses girl
(n) Catcher
