# Supplementary material for: VLMAE: Vision-Language Masked Autoencoder
Source: arXiv:2208.09374 source file (2022-08-19)
Supplement: Supplementary file 2 [file supp_pre.tex]

\begin{table}[h]
\tablestyle{6pt}{1.02}
\footnotesize
\begin{tabular}{y{96}|y{68}}
config & value \\
\shline
image size & 256 \\
max text length & 25 \\
batch size & 512 \\
optimizer & AdamW \\
learning rate & 1e-4 \\
weight decay & 0.02 \\
learning rate schedule & cosine decay \\
epochs & 30 \\
augmentation & RandomCrop, RandAug
\end{tabular}
\caption{\textbf{Pre-training setting.}}
\label{tab:supp_pre}
\end{table}
